# Supplementary material for: Strongly correlated doped hole carriers in the superconducting nickelates: Their location, local many-body state, and low-energy effective Hamiltonian
Source: arXiv:2005.00022 source file (2022-12-14)
Supplement: Supplementary file 1 [file Supplementary.pdf]

# Supplementary materials: Where do the hole carriers go in the new superconducting nickelates?

Zi-Jian Lang, Ruoshi Jiang, and Wei Ku

**Calculation details.** All LDA+ $U$  results were obtained via the linearized augmented plane wave method [S1]. Crystal structure are P4/mmm with lattice constant  $a = b = 3.92\text{\AA}$ ,  $c = 3.37\text{\AA}$ , with  $U - J = 0.6 - 0.06 = 0.54\text{Ry}$  for Ni- $d$  orbital, and 0.2, 0.6Ry for Nd- $d, f$  orbitals. Calculation for antiferromagnetic case uses  $G$ -type spin configuration with  $\sqrt{2} \times \sqrt{2} \times 2$  supercell.

**Effective Hamiltonians at different energy levels.** To obtain a set of realistic parameters in  $H^{eff}$ , we require the Hartree-Fock approximation of our  $H^{eff}$  to reproduce the LDA+ $U$  band structure (or equivalently the Kohn-Sham Hamiltonian) within the subspace of the four active orbitals [S2], including two “inner-shell” orbitals Ni- $d_{x^2-y^2}$ , Ni- $d_{3z^2-r^2}$ , and two “outer-shell” orbitals  $P_a$  and  $P_s$  as anti-symmetric and symmetric superposition of O- $p$  orbitals. This mapping makes sense because the LDA+ $U$  approximation employs a similar treatment of the intra-atomic many-body interactions. Specifically, we obtain  $t_{ij'}$  from the LDA+ $U$  Kohn-Sham Hamiltonian,  $H^{LDA+U}$ , represented in atomic Wannier orbitals [S3].  $J_m$  is calculated from comparing two  $H^{LDA+U}$  of the same magnetic structure but with opposite Nd- $f$  spin direction which is listed in Table S1.

TABLE S1.  $J_m$  in Eq.(1) for four different orbitals.

| orbital          | $d_{x^2-y^2}$ | $d_{3z^2-r^2}$ | $P_a$    | $P_s$    |
|------------------|---------------|----------------|----------|----------|
| $J_m(\text{eV})$ | 0.02          | 0.05           | $\sim 0$ | $\sim 0$ |

We then approximate  $U_{dd'}$  and  $J_{dd'}$  via a Slater integral [S4, S5] with  $U_{eff}$  and  $J_{eff}$ , which are treated as the only fitting parameters. With  $U_{dd'}$ ,  $J_{dd'}$  and  $J_m$  fixed,  $\epsilon_{im}$  can be obtained by subtracting the mean-field of Hartree-Fock and  $J_m$  from the above  $H^{LDA+U}$  and requires both spin channels to have the same value [S2]. In our case,  $U_{eff} = 7.4\text{eV}$ ,  $J_{eff} = 1.2\text{eV}$  (thus,  $U_{d_{x^2-y^2}d_{x^2-y^2}} = 8.8\text{eV}$ ,  $U_{d_{x^2-y^2}d_{3z^2-r^2}} = 6.6\text{eV}$ ) can well reproduce the LDA+ $U$  results. We set the on-site repulsion of oxygen atoms  $U_{pp} = 4\text{eV}$  [S6] in our exact diagonalization process for obtaining the local many-body state. The resulting effective Hamiltonian in different energy scale are listed in Table S2, S3 and S4. Table S4 shows the comparison between nickelates and cuprates.

The leading in-plane and out-of-plane inter-site hopping parameters are listed in Table S5 in order to obtain the kinetic energy for Ni-O spin-singlet and Ni<sup>2+</sup> spin-triplet state.

**Insensitivity to interaction parameters.** To investigate the influence of onsite repulsion  $U$  of Ni  $d$  orbital on the main conclusion that the hole carriers mostly reside in O and spin-majority Ni- $d_{x^2-y^2}$  orbital, we test our conclusion for various of  $U_{eff}$  (from 3eV to 12eV) as shown in Fig. S1. Upon including the kinetic energy  $T$ , the energy difference between the

TABLE S2. Local on-site and kinetic energy in  $H^{eff}$  for Ni- $d_{x^2-y^2}$ ,  $d_{3z^2-r^2}$ , and two O- $p_{\parallel}$  orbitals pointing toward Ni from the two O sites next to Ni.

| $H^{LDA+U}$ (eV)     | $d_{x^2-y^2}$ | $d_{3z^2-r^2}$ | $p_{\parallel}(p_x)$ | $p_{\parallel}(p_y)$ |
|----------------------|---------------|----------------|----------------------|----------------------|
| $d_{x^2-y^2}$        | -3.88         | 0              | -1.37                | 1.37                 |
| $d_{3z^2-r^2}$       | 0             | -3.39          | 0.40                 | 0.40                 |
| $p_{\parallel}(p_x)$ | -1.37         | 0.40           | 5.06                 | 0.65                 |
| $p_{\parallel}(p_y)$ | 1.37          | 0.40           | 0.65                 | 5.06                 |

TABLE S3. Local on-site and kinetic energy in  $H^{eff}$  for inner-shell  $d_{x^2-y^2}$ ,  $d_{3z^2-r^2}$ , and outer-shell  $P_a$ ,  $P_s$  orbitals.

| $H^{eff}$ (eV) | $d_{x^2-y^2}$ | $P_a$ | $d_{3z^2-r^2}$ | $P_s$ |
|----------------|---------------|-------|----------------|-------|
| $d_{x^2-y^2}$  | -4.09         | -2.56 | 0              | 0     |
| $P_a$          | -2.56         | 4.10  | 0              | 0     |
| $d_{3z^2-r^2}$ | 0             | 0     | -3.51          | 0.69  |
| $P_s$          | 0             | 0     | 0.69           | 6.19  |

Ni<sup>2+</sup> spin-triplet and the Ni-O spin-singlet is always larger than 0.8 eV (red curve) which shows little sensitivity to the choice of interaction parameters. This is because the Ni-O spin-singlet state benefits greatly from a strong kinetic energy and a crystal field without apical oxygen, both of which are independent of  $U$ .

**Considerations on the electron pocket.** For the Nd-5 $d$  orbitals, we want to emphasize that there are lots of calculation showing a large electron pockets [S7–S9] but with no explicit experimental evidence. Due to the well-known self-interaction problem, LDA/LDA+ $U$  method will significantly underestimate the band gap by easily an eV scale from the experience of semiconductor (e.g. Si and Ge) or semi-metals (e.g. Fe-based superconductor [S10]). In addition, weakening of kinetic energy and mass enhancement because of 1) scattering against disorder, 2) electronic correlation (including scattering against fluctuating Ni spins) and 3) polaron formation will all reduce the bandwidth of Nd band and Ni-O band, thus increase the band gap between them (in result of smaller hole and electron pockets). For example, as shown in Fig. S2, in

TABLE S4. Comparison of hopping and exchange parameters of  $H^{1B}$  for Nd<sub>1-x</sub>Sr<sub>x</sub>NiO<sub>2</sub> and La<sub>2-x</sub>Sr<sub>x</sub>CuO<sub>4</sub> [S6] in eV.

|                                                    | $t$  | $t'$  | $t''$ | $J$  |
|----------------------------------------------------|------|-------|-------|------|
| Nd <sub>1-x</sub> Sr <sub>x</sub> NiO <sub>2</sub> | 0.31 | -0.07 | 0.06  | 0.11 |
| La <sub>2-x</sub> Sr <sub>x</sub> CuO <sub>4</sub> | 0.40 | -0.07 | 0     | 0.13 |

TABLE S5. The leading in-plane and out-of-plane inter-site hopping parameters (in eV).

| $i-j$ | $t_{d_{3z^2-r^2}P_a}$ | $t_{P_aP_a}$ | $t_{d_{x^2-y^2}d_{3z^2-r^2}}$ | $t_{d_{3z^2-r^2}d_{3z^2-r^2}}$ | $t_{d_{3z^2-r^2}P_s}$ |
|-------|-----------------------|--------------|-------------------------------|--------------------------------|-----------------------|
| (100) | 0.31                  | 0.23         | 0.11                          | $\sim 0$                       | $\sim 0$              |
| (001) | $\sim 0$              | $\sim 0$     | $\sim 0$                      | 0.29                           | -0.16                 |

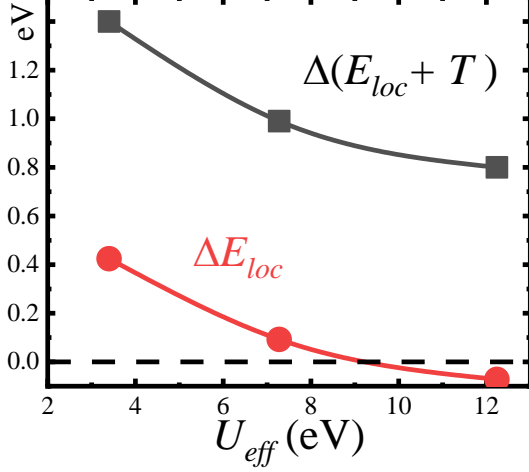

FIG. S1. Energy difference of  $\text{Ni}^{2+}$  spin-triplet and Ni-O spin singlet state as a function of  $U_{\text{eff}}$ . The red curve denotes the difference of local energy of  $\text{Ni}^{2+}$  spin-triplet and Ni-O spin singlet state. Including the large kinetic energy (black curve), the energy of singlet always remains lower even at 12 eV, which is insensitive to the choice of local repulsion.

the antiferromagnetic order phase, the weight of  $\text{Nd}-d_{xy}$  orbital near the Fermi surface is negligibly small compared with Ni orbitals. Therefore, the role of  $\text{Nd}-5d$  orbitals is far from being established. On the other hand, the main interest here is where the hole carriers reside in superconducting samples. Even there are some electrons in  $\text{Nd}-5d$  orbitals in the undoped system, by 20% doping the number of electron carriers would have been largely depleted and negligibly small. And the additional holes (besides the intrinsic holes in Ni) in doped

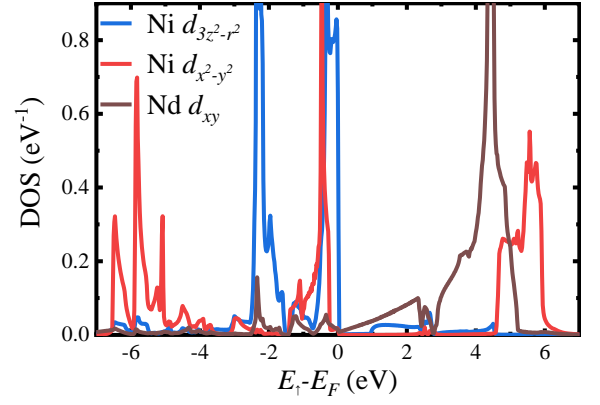

FIG. S2. Density of states (DOS) of different orbitals of the spin majority channel for the AFM phase, where the blue, red and brown line denote the  $\text{Ni}-d_{3z^2-r^2}$ ,  $d_{x^2-y^2}$  and  $\text{Nd}-d_{xy}$  orbitals respectively.

system will still reside in the oxygen orbitals as a part of Ni-O spin-singlet state regardless of whether they are from the self-doping or Sr-doping.

- [S1] V. I. Anisimov, I. V. Solovyev, M. A. Korotin, M. T. Czyżyk, and G. A. Sawatzky, *Phys. Rev. B* **48**, 16929 (1993).
- [S2] W.-G. Yin, D. Volja, and W. Ku, *Phys. Rev. Lett.* **96**, 116405 (2006).
- [S3] W. Ku, H. Rosner, W. E. Pickett, and R. T. Scalettar, *Phys. Rev. Lett.* **89**, 167204 (2002).
- [S4] J. Slater, *Quantum Theory of Molecules and Solids* (McGraw-Hill, New York, 1974).
- [S5] A. I. Liechtenstein, V. I. Anisimov, and J. Zaanen, *Phys. Rev. B* **52**, R5467 (1995).
- [S6] M. Ogata and H. Fukuyama, *Reports on Progress in Physics* **71**, 036501 (2008).
- [S7] K.-W. Lee and W. E. Pickett, *Phys. Rev. B* **70**, 165109 (2004).
- [S8] A. S. Botana and M. R. Norman, *Phys. Rev. X* **10**, 011024 (2020).
- [S9] M.-Y. Choi, K.-W. Lee, and W. E. Pickett, *Phys. Rev. B* **101**, 020503 (2020).
- [S10] A. Tamai, A. Y. Ganin, E. Rozbicki, J. Bacsá, W. Meevasana, P. D. C. King, M. Caffio, R. Schaub, S. Margadonna, K. Prasad, M. J. Rosseinsky, and F. Baumberger, *Phys. Rev. Lett.* **104**, 097002 (2010).
